# Supplementary material for: PIE-NET: Parametric Inference of Point Cloud Edges
Source: arXiv:2007.04883 source file (2020-10-25)
Supplement: Supplementary file 1 [file supp_all_methods.tex]

\begin{figure*}[!t]
\centering
\includegraphics[width=\linewidth]{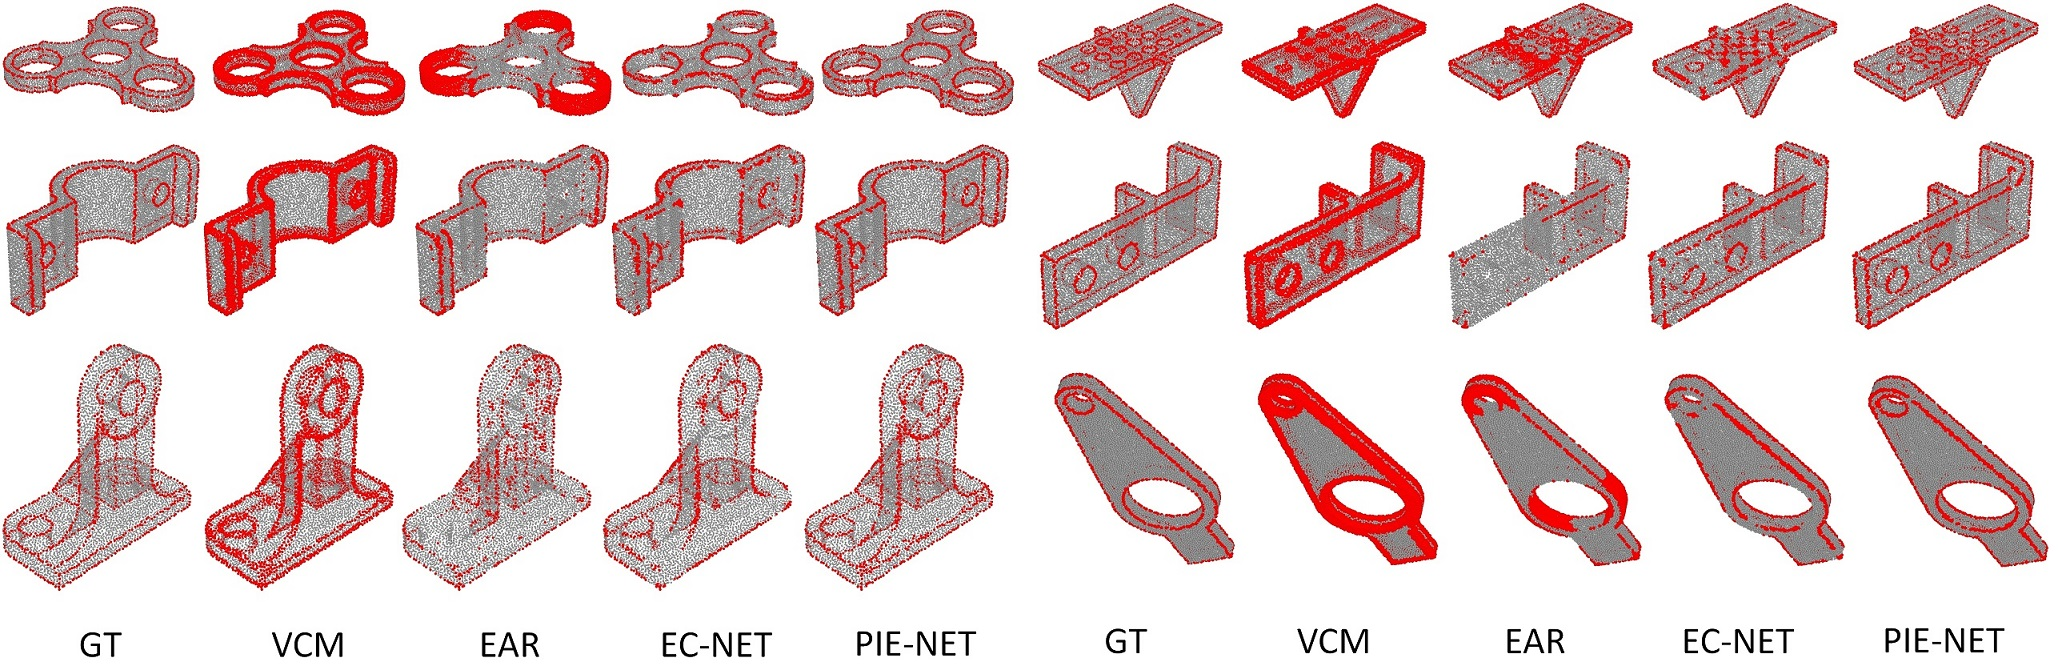}
%\vspace{-2em}
\caption{\textbf{Comparisons to state-of-the-art methods} --
Qualitative comparisons against edge detection techniques -- VCM~\cite{merigot2011}, EAR~\cite{huang2013}, and EC-Net~\cite{yu2018_ECNET}.
}
\label{fig:supp_star}
\end{figure*}
